# Supplementary material for: Symmetry breaking and entropy production during the evolution of spinor Bose-Einstein condensate driven by coherent atom beam
Source: arXiv:1909.08225 source file (2019-09-18)
Supplement: Supplementary file 1 [file Supplementary-1.pdf]

# Supplementary: Magnetization fluctuation of the condensate in early time of scattering with a symmetric incoming atom beam

Yixin Xu[1], Zhongda Zeng[1], Zbigniew Domanski[2], and Zhibing Li[1,3,4*]
[1]*School of Physics, Sun Yat-Sen University, Guangzhou, 510275, P. R. China*
[2]*Institute of Mathematics, Czestochowa University of Technology, 42-201 Czestochowa, Poland*
[3]*State Key Laboratory of Optoelectronic Materials and Technologies, Guangzhou, 510275, P. R. China and*
[4]*Guangdong Province Key Laboratory of Display Material and Technology, Guangzhou, 510275, P. R. China*

PACS numbers: 03.75.Gg;03.75.Kk; 03.75.Mn

The iteration equation for $\lambda_m(n)$ reads

$$\lambda_m(t_n) = \frac{1}{Z(t_n)} \sum_{m'} \sum_{\mu=-1}^{1} |T^{m'}_{m,\mu}|^2 \lambda_{m'}(t_{n-1}) \qquad (1)$$

where

$$\begin{aligned} Z(t_n) \;=\; & \sum_{m,\mu} \lambda_m(t_{n-1}) \{[1 + (C_{m-\mu,\mu})^2]^2 |\xi^i_\mu|^2 \\ & + (C_{m-\mu,\mu\mp1} C_{m-\mu,\mu})^2 |\xi^i_{\mu\mp1}|^2 \\ & (C_{m-\mu,\mu\mp2} C_{m-\mu,\mu})^2 |\xi^i_{\mu\mp2}|^2\} \end{aligned} \qquad (2)$$

is the normalization factor. The squared transition matrix has the following form

$$\begin{aligned} |T^{m'}_{m,\mu}|^2 \;=\; & \delta_{m',m}[1 + (C_{m-\mu,\mu})^2]^2 |\xi^i_\mu|^2 \\ & + \delta_{m',m\pm1} (C_{m'-\mu,\mu\mp1} C_{m'-\mu,\mu})^2 |\xi^i_{\mu\mp1}|^2 \\ & \delta_{m',m\pm2} (C_{m'-\mu,\mu\mp2} C_{m'-\mu,\mu})^2 |\xi^i_{\mu\mp2}|^2 \end{aligned} \qquad (3)$$

with implied summation over $m \mp 1$ and $m \mp 2$.

The Clebsch-Gordan coefficients for coupling the spin states $|S = N-1, m\rangle$ and $|S = 1, \mu\rangle$ into the state $|S = N, m\rangle$ are known as

$$\begin{aligned} C_{m,\mu} \;\equiv\; & C^{N-1,1}_{N,m+\mu;m,\mu} \\ =\; & \mu^2 \left[\frac{(N+\mu m)(N+\mu m+1)}{2N(2N-1)}\right]^{\frac{1}{2}} \\ & + (1-\mu^2) \left[\frac{N^2 - m^2}{N(2N-1)}\right]^{\frac{1}{2}} \end{aligned} \qquad (4)$$

Take the magnetic quantum number per atom $x = m/N$ and its k-*th* moment at $t_n$ defined as

$$\bar{x}_k(t_n) = \frac{1}{N^k Z(t_n)} \sum_m m^k \lambda_m(t_n) \qquad (5)$$

Substitutions of (1) and (3) in (5) give

$$\begin{aligned} & \bar{x}_k(t_n) = \\ & \frac{1}{N^k Z(t_n)} \sum_{m,\mu} \lambda_m(t_{n-1}) \{m^k [1 + (C_{m-\mu,\mu})^2]^2 |\xi^i_\mu|^2 \\ & + (m \mp 1)^k (C_{m-\mu,\mu\mp1} C_{m-\mu,\mu})^2 |\xi^i_{\mu\mp1}|^2 \\ & + (m \mp 2)^k (C_{m-\mu,\mu\mp2} C_{m-\mu,\mu})^2 |\xi^i_{\mu\mp2}|^2\} \end{aligned} \qquad (6)$$

and thus the summations over $m$ in (2) and (6) can be expressed in terms of moments (5) at $t_{n-1}$,

$$\bar{x}_k(t_n) = \frac{\sum_{j=0}^{k+2} g_{k,j} \bar{x}_j(t_{n-1})}{N^k \sum_{j=0}^{2} z_j \bar{x}_j(t_{n-1})} \qquad (7)$$

Consider the condensate having the symmetric initial spin distribution $\lambda_m(0) = \delta_{m,0}$ and the incoming-atom state $|\xi^{0y}|\rangle_a = \frac{1}{\sqrt{2}}(|-1\rangle_a + |1\rangle_a)$. Due to the global spin-reversal symmetry, the magnetization per atom $\bar{x}_1 = 0$, therefore $\bar{x}_2 = \chi$ is the fluctuation of $x$,

$$\chi(t_n) = \frac{g_{2,0} + g_{2,2}\chi(t_{n-1}) + g_{2,4}\bar{x}_4(t_{n-1})}{N^2(z_0 + z_2\chi(t_{n-1}))} \qquad (8)$$

Using (4), we obtain following prefactors of $\chi(t_{n-1})$ and $\bar{x}_j(t_{n-1})$ in RHS of (8):

$$z_0 = -1 + 4N - 13N^2 + 14N^3 \qquad (9)$$
$$z_2 = 3N - 7N^2 + 6N^3 \qquad (10)$$
$$g_{2,0} = -4 - 2N + 5N^2 + 3N^3 \qquad (11)$$
$$g_{2,2} = 14N - 14N^2 - 6N^3 - 9N^4 + 14N^5 \qquad (12)$$
$$g_{2,4} = 10N^3 - 11N^4 + 6N^5 \qquad (13)$$

For $N \gg 1$, $\chi(t_n)$ can be approximated by a continuous function of $t_n$ and differences of $\chi$ between consecutive scatterings approach the derivative

$$\frac{d\chi(t_n)}{dt_n} \approx \chi(t_n) - \chi(t_{n-1}) \qquad (14)$$

Relations (9)-(14) enable us to transform (8) into following differential equation

$$\frac{d\chi}{dt} = \frac{g_{2,0} + (g_{2,2} - N^2 z_0)\chi + g_{2,4}\bar{x}_4 - N^2 z_2 \chi^2}{N^2(z_0 + z_2\chi)} \qquad (15)$$

*Corresponding author: Z.B.Li, stslzb@mail.sysu.edu.cn

In the early-time, the fluctuation is small and one can neglect cumulants of order higher than two. Since $\bar{x}_4 = 3\chi^2$ then (15) becomes

$$\frac{d\chi}{dt} = \frac{g_{2,0} + (g_{2,2} - N^2 z_0)\chi + (3g_{2,4} - N^2 z_2)\chi^2}{N^2(z_0 + z_2\chi)} \quad (16)$$

Making use of (9-13) and up to the leading order of $N$, (16) can be further approximated by

$$\frac{d\chi}{dt} = \frac{12\chi^2}{14 + 6\chi} \quad (17)$$

The integration of (17) yields

$$\frac{7}{6\chi(t_0)} - \frac{7}{6\chi(t)} + \frac{1}{2}\ln\frac{\chi(t)}{\chi(t_0)} = t - t_0 \quad (18)$$

Neglecting the small logarithmic term, one obtains

$$\chi(t) = \frac{\chi(t_0)}{1 - \frac{6}{7}\chi(t_0)(t - t_0)} \quad (19)$$
